# Supplementary material for: DiTTo-TTS: Diffusion Transformers for Scalable Text-to-Speech without Domain-Specific Factors
Source: arXiv:2406.11427 source file (2025-02-17)
Supplement: Supplementary file 1 [file appendix_additional_architecture_search_1.tex]

\begin{table}[ht]
  \caption{Performances of English-only cross-sentence task from the additional architecture search. All settings are consistent with those outlined in Section~\ref{sec:}.
  Results confirm the effectiveness of the architectural design of our model. The boldface indicates the best result.
  }
  \label{tab:appendix_additional_architecture_search}
  \centering
  \begin{tabular}{lllll}
    \toprule
    \bf Model & \bf WER\ $\downarrow$ & \bf SIM-r\ $\uparrow$ & \makecell{\bf Codec\\ \bf PESQ $\uparrow$} & \makecell{\bf Codec\\ \bf ViSQOL $\uparrow$} \\
    \midrule
    DiTTo-\textit{dac-24k-scale-shift-0.1}          & 4.78 & 0.5098 & \multirow{3}{*}{\bf 4.37} & \multirow{3}{*}{\bf 4.91} \\
    DiTTo-\textit{dac-24k-scale-shift-0.2}          & 4.70 & 0.5362 &  &  \\
    DiTTo-\textit{dac-24k-scale-shift-0.3}          & 7.21 & 0.5545 &  &  \\
    \midrule
    DiTTo-\textit{dac-44k-scale-shift-0.1}          & 7.70 & 0.5366 & \multirow{3}{*}{\underline{3.74}} & \multirow{3}{*}{\underline{4.85}} \\
    DiTTo-\textit{dac-44k-scale-shift-0.2}          & 8.71 & 0.5428 &  &  \\
    DiTTo-\textit{dac-44k-scale-shift-0.3}          & 14.58 & 0.5597 &  &  \\
    \midrule
    DiTTo-\textit{no-pooled-text}                   & 3.00 & 0.5791 & \multirow{3}{*}{2.95} & \multirow{3}{*}{4.66} \\
    DiTTo (from Table~\ref{tab:ab_model_architecture})& \bf 2.93 & \underline{0.5877} &  &  \\
    DiTTo-\textit{no-rvq-decoding}                  & \underline{2.97} & \bf 0.5883 &  &  \\
    \bottomrule
  \end{tabular}
\end{table}
